# Supplementary material for: CellTypeGraph: A New Geometric Computer Vision Benchmark
Source: arXiv:2205.08166 source file (2022-05-17)
Supplement: Supplementary file 1 [file graph_feat.pdf]

# Graph Features

Class-average Accuracy

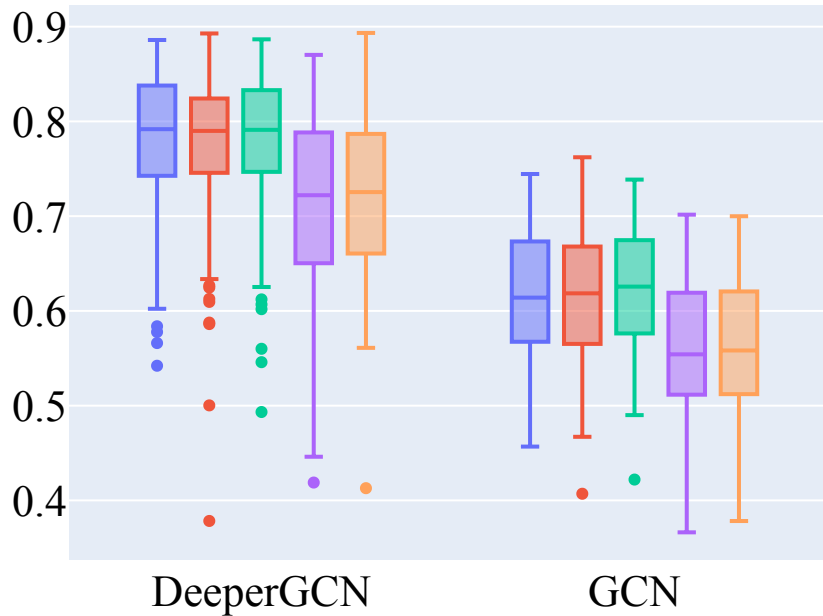

- Onehot [-1, 1]. Quantile Clipping + Zscore
- Onehot [0, 1], Graph feat. Quantile Clipping + Zscore
- Graph feat. Zscore
- Graph feat. Quantile Clipping
- Graph feat. Base
